# Supplementary material for: SE(3) diffusion model with application to protein backbone generation
Source: arXiv:2302.02277 source file (2023-05-22)
Supplement: Supplementary file 1 [file sde_se3.tex]

% \section{Forward and time-reversal on $\SE(3)$}
\section{SDE on $\SE(3)$}
\todo[inline]{To merge with \cref{sec:laplacian-se_3rset}}
\label{sec:forw-time-revers}

\subsection{The $\SE(3)$ group} \label{sec:}

\paragraph{Euclidean group} \label{sec:def_se3}
The Euclidean group $\E(n)$ is the group of isometries of a Euclidean space $\R^n$: $\E(n) \triangleq \text{Isom}(\mathbb{R}^n)$.
We have that $\E(n)= \T(n) \ltimes \O(n)$, with $\T(n) \cong \R^n$ the group of translation and $\O(n) = \{R \in \GL(n, \R)| R^\top R = R R^\top = I\}$ the orthogonal group.
$\O(n)$ and thus $\E(n)$ have two components, one consists of all orthogonal matrices of determinant $1$ and the other component with determinant $-1$.

\paragraph{Special Euclidean group}
Let's focus on $\SE(n) = \T(n) \ltimes \SO(n)$ which is simply connected.
$\T(n) \triangleleft~ \SE(n)$ is a normal subgroup---that is
$g^{-1}pg \in \T(n)$ for any $p \in \T(n), g \in \SE(n)$, while
$\SO(n)=\{R \in GL(n)| R^\top R = I, \det R = 1\}$ is a (non-normal) subgroup of
$\SE(n)$.  The group operator between two elements $T=(R, x) \in \SE(n)$ and
$T'=(R', x') \in \SE(n)$ is defined as $T \cdot T' = (R R', R x' + x)$, and the
group inverse operator is defined by $T^{-1} = (T^\top, - R^\top x)$.  We see
that $\SE(n)$ is \emph{not} the direct product between $\T(n)$ and $\SO(n)$ as
otherwise we would have that $T \cdot T' = (R R', x' + x)$ and
$T^{-1} = (T^\top, -x)$.  Using homogenous coordinates, $\SE(3)$ can be
represented as follow
$$\SE(3) = \biggl\{
\begin{bmatrix}
    R & x \\
    \mathbf{0}^\top & 1
  \end{bmatrix} \in \GL(4, \R)| R \in \SO(3), x \in \R^3 
  \biggr\}.$$
Then the group operator `$\cdot$' is simply the matrix multiplication, and the group inverse is the matrix inverse.

In this section, we consider a forward process on $\SE(3)$ given by a
Brownian motion on $\SO(3)$ and a Brownian motion on $\rset^3$.
