# Supplementary material for: SE(3) diffusion model with application to protein backbone generation
Source: arXiv:2302.02277 source file (2023-05-22)
Supplement: Supplementary file 2 [file IGSO3_example_main_file.tex]

\documentclass{article}
\usepackage{listings}
\usepackage{icml2023}
\usepackage{xcolor}
\input{content/macros}
\begin{document}

\onecolumn
\input{content/appendix/IGSO3_example_main}

\end{document}
